# Supplementary material for: The energy scale of Dirac electrons in Cd3As2
Source: arXiv:1803.05469 source file (2018-03-14)
Supplement: Supplementary file 1 [file SupplementaryMaterials.pdf]

# Supplementary Materials for "The energy scale of Dirac electrons in $Cd_3As_2$"

M. Hakl,[1,*] S. Tchoumakov,[2] I. Crassee,[1] A. Akrap,[3] B. A. Piot,[1] C. Faugeras,[1] G. Martinez,[1] A. Nateprov,[4] E. Arushanov,[4] F. Teppe,[5] R. Sankar,[6,7] Wei-li Lee,[6] J. Debray,[8,9] O. Caha,[10] J. Novák,[10] M. O. Goerbig,[2] M. Potemski,[1] and M. Orlita[1,11,†]

[1] *Laboratoire National des Champs Magnétiques Intenses, CNRS-UGA-UPS-INSA, 25, avenue des Martyrs, 38042 Grenoble, France*
[2] *LPS, Univ. Paris-Sud, Univ. Paris-Saclay, CNRS UMR 8502, 91405 Orsay, France*
[3] *DQMP, University of Geneva, 1211 Geneva 4, Switzerland*
[4] *Institute of Applied Physics, Academy of Sciences of Moldova, 2028 Chisinau, Moldova*
[5] *Laboratoire Charles Coulomb, CNRS, Université Montpellier, 34095 Montpellier, France*
[6] *Institute of Physics, Academia Sinica, Nankang, 11529 Taipei, Taiwan*
[7] *Center for Condensed Matter Sciences, National Taiwan University, Taipei 10617, Taiwan*
[8] *Université Grenoble Alpes, Institut NEEL, F-38000 Grenoble, France*
[9] *CNRS, Institut NEEL, F-38000 Grenoble, France*
[10] *CEITEC MU and Faculty of Science, Masaryk University, 61137 Brno, Czech Republic*
[11] *Institute of Physics, Charles University, Ke Karlovu 5, 12116 Praha 2, Czech Republic*

In these Supplementary Materials, we provide details about calculations of the Landau level spectrum within the Bodnar model, assuming that the magnetic field $B$ is oriented along the (112) crystallographic direction. We also present a comparison of our experimental data with expectations of the simple Kane model, which completely neglects the influence of the crystal-field splitting parameter $\delta$.

## LANDAU LEVEL QUANTIZATION FOR (112)-ORIENTATED BODNAR HAMILTONIAN

Due to the anisotropy of the electronic band structure implied by the Bodnar model, which is best visible at relatively low energies and which is closely related to the possible appearance of Dirac cones, the corresponding Landau level spectrum depends on the particular orientation of the applied magnetic field. The simplest case, with $B$ oriented along the tetragonal (001) axis was reviewed in the context of our preceding cyclotron resonance study [1]. Here we present calculations for the magnetic field oriented along the (112) direction, which is the natural direction of $Cd_3As_2$ growth/cleavage and which is also relevant for the magneto-transmission experiment presented in the main part of this work. Let us also note that the (112) direction within the full unit cell of $Cd_3As_2$ corresponds to the (111) direction within the simplifying anti-fluorite lattice considered by Bodnar [2].

In the magnetic field, which is applied along a generally oriented unit vector $(\sin\theta,\, 0,\, \cos\theta)^{\mathsf{T}}$, the commutation relations satisfy:

$$[k_x,\, k_y] = -\frac{i}{l_B^2}\cos\theta,\; [k_x,\, k_z] = 0,\; [k_y,\, k_z] = -\frac{i}{l_B^2}\sin\theta\,. \tag{1}$$

Using these commutation relations in the Bodnar model [3], the Landau level spectrum may be calculated from the implicit equation:

$$\gamma(E_n) = \frac{\mathrm{sgn} f_1(E_n)(2n+1)}{l_B^2}\sqrt{f_1(E_n)(\cos^2\theta f_1(E_n) + \sin^2\theta f_2(E_n))} + \frac{f_1(E_n) f_2 E_n}{\cos^2\theta f_1(E_n) + \sin^2\theta f_2(E_n)} k_z^2 \pm \frac{P_\perp \Delta}{3 l_B^2}\sqrt{(E_n+\delta)^2 P_\perp^2 \cos^2\theta + E_n^2 P_\parallel^2 \sin^2\theta} \tag{2}$$

where the auxiliary functions $\gamma,\, f_1, f_2$ are defined as

$$\begin{aligned}\gamma(E) &= E(E-E_g)[E(E+\Delta)+\delta(E+\tfrac{2}{3}\Delta)]\,,\\ f_1(E) &= P_\perp^2[E(E+\tfrac{2}{3}\Delta)+\delta(E+\tfrac{1}{3}\Delta)]\,,\\ f_2(E) &= P_\parallel^2 E(E+\tfrac{2}{3}\Delta)\end{aligned} \tag{3}$$

and where the anisotropic Kane parameters, $P_\perp$ and $P_\parallel$ are related to the (anisotropic) velocity parameter as $v_{\perp,\parallel} = \sqrt{\frac{2}{3}} P_{\perp,\parallel}/\hbar$. The signs (+) and (-) refer to the spin set up and down, respectively. The above equation is valid

outside the interval of energies $-\tan^2\theta < f_1(E_n)/f_2(E_n) < 0$ that covers the region of the heavy-hole band for $\delta > 0$. The corresponding eigenfunctions take the standard form $\Psi = (\psi_j)_{j=1..8}$ where each component $\psi_j = a_j \left|n\right\rangle_j u_j$ is expressed just by a single harmonic function $\left|n\right\rangle_j$ and a basis vector $u_j$.

Another possible approach is to rotate the whole Bodnar Hamiltonian into a new coordination system, in which the $z$-axis coincides with the direction of the applied magnetic field: $\boldsymbol{B} = (0,0,B)^{\mathsf{T}}$. This can be done by rescaling and rotation of the momentum coordinates $q_x$, $q_y$, $q_z$ through the following transformation:

$$\begin{pmatrix} q_x \\ q_y \\ q_z \end{pmatrix} = \begin{pmatrix} \frac{P_\perp}{P}\cos\xi & 0 & -\frac{P_\parallel}{P}\sin\xi \\ 0 & \frac{P_\perp}{P} & 0 \\ \frac{P_\perp}{P}\sin\xi & 0 & \frac{P_\parallel}{P}\cos\xi \end{pmatrix} \begin{pmatrix} k_x \\ k_y \\ k_z \end{pmatrix} . \tag{4}$$

The new commutation relations then take the form:

$$[q_x, q_y] = -\frac{i}{l_B^2}\left(\frac{P_\perp^2\cos(\xi)\cos(\theta) + P_\perp P_\parallel \sin(\xi)\sin(\theta)}{P^2}\right), \ [q_x, q_z] = 0, \ [q_y, q_z] = \frac{i}{l_B^2}\frac{P_\perp}{P}\left[\frac{P_\perp}{P}\cos(\theta)\sin(\xi) - \frac{P_\parallel}{P}\cos(\xi)\sin(\theta)\right] . \tag{5}$$

which we simplify choosing $\xi$ and $P$ such that

$$P = \sqrt{|P_\perp^2\cos(\xi)\cos(\theta) + P_\perp P_\parallel \sin(\xi)\sin(\theta)|}, \tag{6}$$

$$\xi = \arctan\left[\frac{P_\perp}{P_\parallel}\tan(\theta)\right] . \tag{7}$$

This way one finds

$$[q_x, q_y] = -\frac{i}{l_B^2}, \ [q_x, q_z] = 0, \ [q_y, q_z] = 0. \tag{8}$$

The corresponding Hamiltonian undergoes a unitary transformation $\hat{H}_\xi = U_\xi^{-1}\hat{H}U_\xi$ and reads (in its matrix form):

$$\begin{pmatrix} E_g & Pq_- & -Pq_+ & 0 & 0 & 0 & 0 & Pq_z \\ Pq_+ & -\frac{\delta\sin^2(\xi)}{2} & \frac{\delta\sin^2(\xi)}{2} & 0 & 0 & 0 & 0 & \frac{\delta\sin(2\xi)}{2\sqrt{2}} \\ -Pq_- & \frac{\delta\sin^2(\xi)}{2} & -\frac{\delta\sin^2(\xi)}{2} - \frac{2}{3}\Delta & \frac{\sqrt{2}\Delta}{3} & 0 & 0 & 0 & -\frac{\delta\sin(2\xi)}{2\sqrt{2}} \\ 0 & 0 & \frac{\sqrt{2}\Delta}{3} & -\delta\cos^2(\xi) - \frac{\Delta}{3} & Pq_z & \frac{\delta\sin(2\xi)}{2\sqrt{2}} & \frac{\delta\sin(2\xi)}{2\sqrt{2}} & 0 \\ 0 & 0 & 0 & Pq_z & E_g & Pq_+ & Pq_- & 0 \\ 0 & 0 & 0 & \frac{\delta\sin(2\xi)}{2\sqrt{2}} & Pq_- & -\frac{\delta\sin^2(\xi)}{2} & -\frac{\delta\sin^2(\xi)}{2} & 0 \\ 0 & 0 & 0 & \frac{\delta\sin(2\xi)}{2\sqrt{2}} & Pq_+ & -\frac{\delta\sin^2(\xi)}{2} & -\frac{\delta\sin^2(\xi)}{2} - \frac{2}{3}\Delta & \frac{\sqrt{2}\Delta}{3} \\ Pq_z & \frac{\delta\sin(2\xi)}{2\sqrt{2}} & -\frac{\delta\sin(2\xi)}{2\sqrt{2}} & 0 & 0 & 0 & \frac{\sqrt{2}\Delta}{3} & -\delta\cos^2(\xi) - \frac{\Delta}{3} \end{pmatrix} \tag{9}$$

with the corresponding LS-basis:

$$(s\uparrow, u_{-1}\uparrow, u_0\uparrow, u_{+1}\uparrow, s\downarrow, u_{-1}\downarrow, u_0\downarrow, u_{+1}\downarrow) , \tag{10}$$

where $u_n$ functions are built for $L = 1$ as:

$$u_{-1} = \frac{i}{\sqrt{2}}(u_x - iu_y), \ u_0 = iu_z, \ u_1 = \frac{-i}{\sqrt{2}}(u_x + iu_y) . \tag{11}$$

When we introduce the magnetic field into the above Hamiltonian, via standard ladder operators, one may conclude that no simple eight-component vector can satisfy all ladder operations in the eigenproblem $H_{(112)}\Psi = E\Psi$ at once and a more general ansatz, using a perturbative approach for the each component of the wavefunction $\Psi = (\psi_j)_{j=1..8}$, needs to be chosen:

$$\psi_j = \sum_{n=0}^{N_{\max}} a_{j,n}\left|n\right\rangle , \tag{12}$$

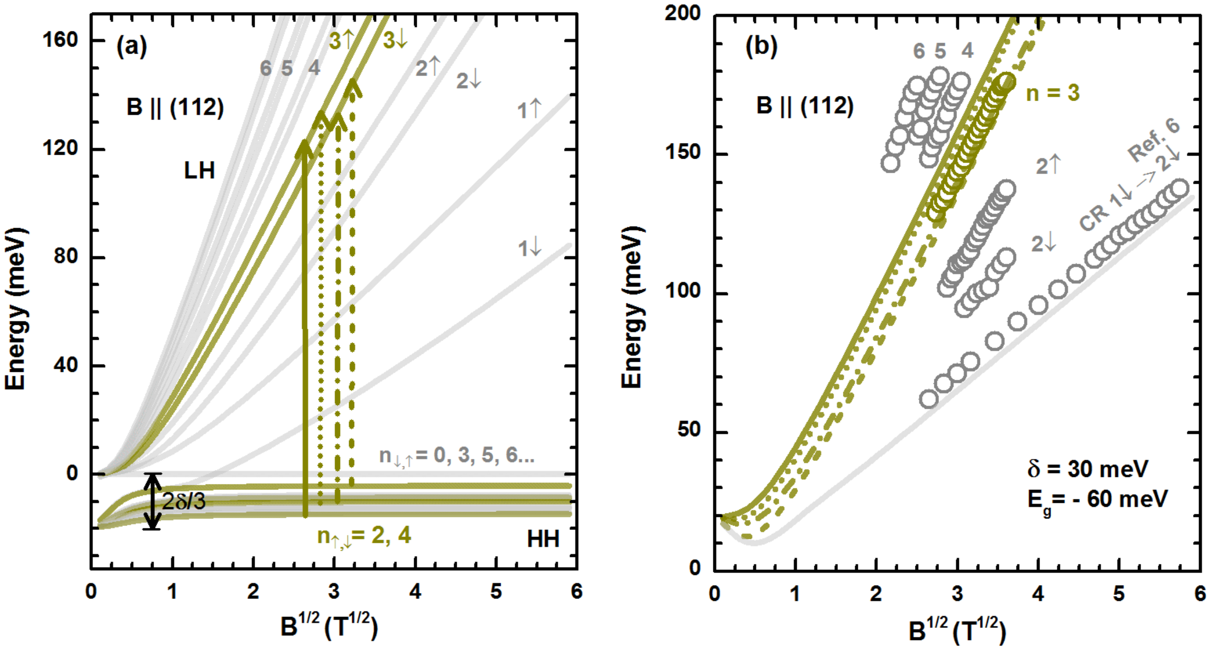


FIG. 1. (a) Landau level spectrum calculated within the Bodnar model for $E_g = -60$ meV and $\delta = 30$ meV with the magnetic field oriented along the (112) direction. The vertical arrows denote the quadruplet of inter-Landau level transitions from the flat band to the upper conical band with the final-state level $n = 3$. (b) the experimental position of observed resonances compared to the theoretically expected transition energies calculated from (a).

where $N_{\max}$ stands for the order of the expansion. Using this ansatz, we finally end up with the following set of eight equations:

$$\sum_{j=1}^{8} \sum_{n=0}^{N_{\max}} H_{ij}\, a_{j,n} \left|n\right\rangle = E \sum_{n=0}^{N_{\max}} a_{j,n} \left|n\right\rangle \ . \tag{13}$$

When each equation is projected out by one of the harmonic function $\langle n'|_{n'=1..N_{max}}$ in the solution (12), the coefficients $a_{j,n}$ can be obtained as:

$$\sum_{j=1}^{8} \sum_{n=0}^{N_{\max}} \langle n'|H_{ij}|n\rangle \ a_{j,n} = E \sum_{n=0}^{N_{\max}} a_{j,n}\delta_{n',n} \, . \tag{14}$$

Altogether, the set of $N_{\max} \times 8$ equations (14) provides us with the energies of $N_{\max}$ Landau levels for each from the eight bands.

## COMPARING THEORETICAL ENERGIES OF INTER-LANDAU LEVEL EXCITATIONS WITH EXPERIMENTS

Having calculated the Landau level spectrum, we may compare the expected energies of inter-Landau level excitations with positions of excitations identified experimentally. In this comparison (see Fig. 5 in the main text), we have considered the standard $n \pm 1 \to n$ selection rules, typical of electric-dipole active excitations in systems with an isotropic band structure. Strictly speaking, one may expect a richer excitation spectrum in systems with an anisotropic band structure, implying an additional set of electric-dipole-active excitations, which go beyond these simple selection rules. This fact may be illustrated, for instance, on the complex cyclotron resonance response of $K$ point electrons in bulk graphite, which is characterized by a strongly anisotropic Fermi surface [4]. In the case of $Cd_3As_2$, however, the anisotropy of the electronic band structure is relatively weak [1, 2], and therefore, one may expect that the transitions following the $n \pm 1 \to n$ selection rules dominate the magneto-optical response.

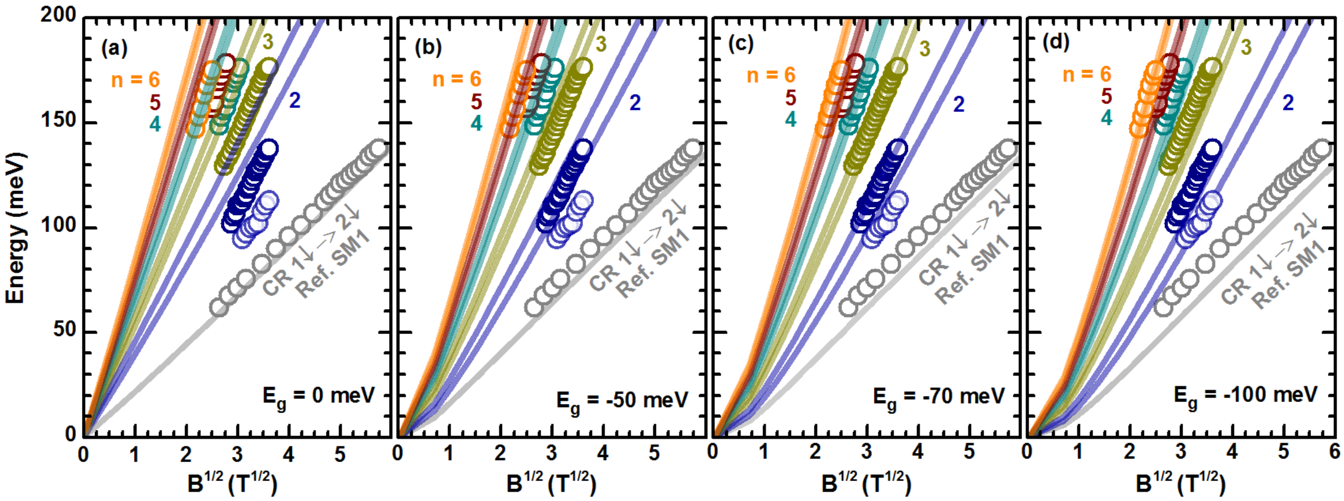


FIG. 2. A comparison of experimental data with theoretically expected positions of resonances calculated within the Kane model ($\delta = 0$) for several values of the (inverted) band gap $E_g = 0, -50, -70$ and -100 meV. The color coding is the same as in Fig. 5 of the main text. The best agreement is found for the band gap around $E_g \approx -70$ meV, which allows us to reproduce the experimental data for both, cyclotron resonance response [1] and interband inter-Landau level resonances, with a reasonable precision.

Staying with the $n \pm 1 \rightarrow n$ selections and focusing on excitations relevant for our experiment – from the flat band to the upper conical band – we get a pair of excitations into each final-state Landau level in the conduction band with a given spin projection $n_{\uparrow,\downarrow}$. For each Landau level index $n$, we thus get altogether four excitations from the flat band to the upper conical band: due to spin splitting of levels in the conduction band and due to the degeneracy of the flat band, which is removed by a non-zero crystal field splitting parameter $\delta$. We illustrate this in Fig. S1 for the case of excitations with the final state in the Landau level $n = 3$. An exemption appears only for the final-state $n = 2$ level, for which only a single pair of excitations: $3\uparrow \rightarrow 2\uparrow$ and $3\downarrow \rightarrow 2\downarrow$, emerges. This is because the $n = 1$ levels are completely missing in the spectrum of the flat band [5].

In the main text, we compare the theoretically calculated excitation energies with our experimental data. All four transitions for each final-state LL $n = 3, 4, 5$ and 6 and two for $n = 2$ have been plotted in Figs. 5a-c. The corresponding color coding facilitates the association of the theoretical lines with the experimental points (see Fig. 5d of the main text). We conclude that the only for $n = 2$ final-state level clear splitting of lines is observed. For $n > 2$, the quadruples of excitations seems to be smeared due to finite widths of individual line. The absence of splitting may be considered as another indication of relatively small $\delta$ parameter in $Cd_3As_2$.

Having concluded small crystal field splitting parameter $\delta$, we may finish our discussion by the comparison of our experimental data with predictions of the (gapped) Kane model. In this case, it is the band gap $E_g$, which remains to be the only tunable parameter, since the velocity parameter is fixed at the value of $v = 0.94 \times 10^6$ m/s known from preceding experimental studies [1, 2, 6]. The theoretically expected energies of inter-Landau level excitations for four different values of the band gap: $E_g = 0, -50, -70$ and -100 meV, have been plotted in Figs. 2a-d and directly compared to the experimental data. Clearly, good agreement is achieved for the band gap values close to $-70$ meV. As one may expect, those are interband excitations which are more sensitive to $E_g$. Interestingly, the band gap value of $E_g = -70$ meV represents a certain trade-off, which compromises the agreement of the theoretical lines with the intraband (cyclotron resonance) data [1] and interband excitations (from magneto-transmission experiments presented in this work).

---

* michaelhakl@email.cz
† milan.orlita@lncmi.cnrs.fr

[1] A. Akrap, M. Hakl, S. Tchoumakov, I. Crassee, J. Kuba, M. O. Goerbig, C. C. Homes, and et al. Magneto-optical signature of massless Kane electrons in cd3as2. *Phys. Rev. Lett.*, 117:136401, 2016.
[2] J. Bodnar. Band structure of cd3as2 from shibnikov-de hass and de hass-alphen effects. In J. Rauluszkiewicz, M. Górska, and E. Kaczmarek, editors, *Proc. III Conf. Narrow-Gap Semiconductors, Warsaw*, page 311. Elsevier, 1977.

[3] P. R. Wallace. Electronic g-factor in $Cd_3As_2$. *Physica Status Solidi (b)*, 92(1):49–55, 1979.
[4] M. Orlita, P. Neugebauer, C. Faugeras, A.-L. Barra, M. Potemski, F. M. D. Pellegrino, and D. M. Basko. Cyclotron motion in the vicinity of a lifshitz transition in graphite. *Phys. Rev. Lett.*, 108:017602, Jan 2012.
[5] M. Orlita, D. M. Basko, M. S. Zholudev, F. Teppe, W. Knap, V. I. Gavrilenko, N. N. Mikhailov, S. A. Dvoretskii, P. Neugebauer, C. Faugeras, A-L. Barra, G. Martinez, and M. Potemski. Observation of three-dimensional massless kane fermions in a zinc-blende crystal. *Nature Phys.*, 10:233, 2014.
[6] Sangjun Jeon et al. Landau quantization and quasiparticle interference in the three-dimensional dirac semimetal cd3as2. *Nature Mater.*, 13:851–856, 2014.
